# Supplementary material for: ClickVOS: Click Video Object Segmentation
Source: arXiv:2403.06130 source file (2024-03-10)
Supplement: Supplementary file 1 [file supplementary.tex]

% \section{Supplementary}


% \subsection{ClickVOS Task}

% \subsubsection{Target Object in ClickVOS}
% With the advancement of interactive segmentation methods, there has been a rise in efforts focusing on segmenting objects at different levels of granularity, such as segmentation for whole or part. It is noted that ClickVOS primarily concerns the whole object granularity. For instance, if a click is placed on a person, the segmentation should encompass the entire person rather than specific body parts like the head or limbs. This maintains consistency with the VOS task and the associated dataset, enabling a fair and convenient exploration of the effect of substituting mask interaction with a single point. Additionally, ClickVOS offers the flexibility for algorithms to concentrate on parts. In ClickVOS, it's possible to flexibly select objects by clicking on background points to suppress the foreground (points indicating other objects can also be considered as background points for the current object).

% \subsubsection{Challenges of ClickVOS}
% Despite the practical significance shown by ClickVOS, it is considered to be a more challenging task. In contrast to SemiVOS, the first frame only provides points to indicate the object instead of the precise mask. It is difficult to determine the appearance of the object to be segmented, which also makes it difficult to use the first frame as an accurate template for matching. Compared with UnVOS, instead of segmenting only the most salient object of the video, it has to segment arbitrary objects according to the custom requirements.


% \subsection{Evaluation and Comparision}

% More qualitative results of the proposed approach on the DAVIS17-P dataset are provided in Fig.~\ref{fig_results_supp}.

% \begin{table}[h]
% \caption{Mask token selection in SAM-based baselines.}
% \centering
% \begin{tabular}{c|c|ccc}
% \toprule
% Method                        & Mask Token  &\(\mathcal{J\&F}\)&\(\mathcal{J}\)&\(\mathcal{F}\)\\
% \midrule
% \multirow{4}{*}{BL-SAM-PT}    & unambiguous & 30.3 & 28.1 & 32.4 \\
%                               & subpart     & 21.5 & 18.4 & 24.7 \\
%                               & part        & 40.5 & 37.5 & 43.4 \\
%                               & whole       & 58.5 & 55.8 & 61.3 \\
% \midrule
% \multirow{5}{*}{BL-SAM-Track} & confident   & 53.8 & 51.4 & 56.3 \\
%                               & unambiguous & 49.1 & 46.4 & 51.9 \\
%                               & subpart     & 40.2 & 37.8 & 42.5 \\
%                               & part        & 49.8 & 46.9 & 53.7 \\
%                               & whole       & 66.3 & 63.3 & 69.3 \\ 
% \bottomrule
% \end{tabular}
% \label{tab_ablation_sam_token}
% \end{table}

% \subsubsection{Tokens Selection in SAM-PT and SAM-track}

% In baseline BL-SAM-PT and BL-SAM-Track, the segmentation model SAM is employed to segment the object mask. And in order to adapt to the different granularity of the target, SAM generates four tokens for each point prompt, which tend to segment the default region (unambiguous token), the whole object (whole token), the subpart (whole token), and the subpart (subpart token). We evaluated the performance of ClickVOS when using different tokens. The BL-SAM-Track implementation also provides an additional option: dynamically selecting the token with the higher SAM-predicted IoU Score. The experimental results show that using the token that tends to split out the whole object is the best in ClickVOS. 
% So we choose the best performance they achieved when using whole-token to participate in the comparison experiment.


% \subsubsection{Objects Perception}

% To evaluate the proposed SegAttn, which percept objects in the first frame by the simple attention, we compare the segmentation quality in the first frame with other segmentation models employed in baselines.
% Specifically, the BL-InterVOS approach adopts fBRS, BL-SemiVOS utilizes MaskRCNN, and BL-SAM-Track and BL-SAM-PT employ the foundational models SAM-Base and SAM-Huge, respectively. As illustrated in Fig.~\ref{fig_f0} and Tab.~\ref{tab_f0_comparison}, in the case where a point can only provide location information, our SegAttn simply and effectively accomplishing object perception is even not inferior to other baselines that employ interactive segmentation models, even in challenging scenarios such as background interference and multiple similar objects. Moreover, our approach won't lose target objects, compared with BL-SemiVOS which employs the instance segmentation model MaskRCNN to predict all possible objects first, followed by the mask selection with points.

% \begin{table}[]
% \centering
% \caption{Comparison of objects perception in the first frame.}
% \begin{tabular}{l|ccc}
% \toprule
% \multicolumn{1}{c|}{Method} &\(\mathcal{J\&F}\)&\(\mathcal{J}\)&\(\mathcal{F}\)\\
% \midrule
% % BL-UnVOS                   &      &      &      \\
% BL-InterVOS                & 73.6 & 68.8 & 78.5 \\
% BL-SemiVOS                 & 66.1 & 63.7 & 68.6 \\
% BL-SAM-Track               & 66.5 & 62.3 & 70.6 \\
% BL-SAM-PT                  & 78.9 & 76.1 & 81.8 \\
% Ours                       & 73.8 & 69.9 & 77.7 \\
% \bottomrule
% \end{tabular}
% \label{tab_f0_comparison}
% \end{table}




% \subsection{Point Annotation}

% We evaluate our model with different points of the first frame in Table \ref{tab_ablation_point}. Overall, our method does not rely on specific points containing the human prior, and it can perform just as well with random points automatically selected from object masks. Manual clicks work slightly better in the multi-object benchmark, and even random points achieved higher performance for the single-object benchmark. These results also highlight the reasonableness of the automatically selected point annotation we provided for the training phase, which not only can reduce the need for human labour but also can ensure that the trained model is robust to points and won't rely on points with specific prior.

% \begin{table}[h]
%     \centering
%     \caption{Ablation study on click points used in inference.}
%     \begin{tabular}{c|ccc}
%     \toprule
%     \multirow{2}{*}{Point Annotation} & \multirow{2}{*}{\begin{tabular}[c]{@{}c@{}}D16\\ \(\mathcal{J\&F}\)\end{tabular}} & \multirow{2}{*}{\begin{tabular}[c]{@{}c@{}}D17\\ \(\mathcal{J\&F}\)\end{tabular}} & \multirow{2}{*}{\begin{tabular}[c]{@{}c@{}}Y19\\ \(\mathcal{J\&F}\)\end{tabular}} \\
%                                       &                                                                                   &                                                                                   &                                                                                 \\
%     \midrule
%     Manual Click              & 85.0 & \textbf{67.6} & \textbf{43.9}\\
%     Automatical from Mask    & \textbf{86.7} & 64.2 & 40.8\\ 
%     \bottomrule
%     \end{tabular}
%     \label{tab_ablation_point}
% \end{table}


% \begin{figure*}[t]
%     \centering
%     \includegraphics[width=1.0\linewidth]{figures/fig_results_supp.pdf}
%     \caption{More qualitative results of the proposed approach on DAVIS17-P dataset.}
%     \label{fig_results_supp}
% \end{figure*}
